# Supplementary material for: Direct Observation of Attractive Skyrmions and Skyrmion Clusters in the Cubic Helimagnet Cu$_2$OSeO$_3$
Source: arXiv:1704.06876 ancillary file (2018-03-21)
Supplement: Supplementary file 1 [file supp.pdf]

# Direct Observation of Attractive Skyrmions and Skyrmion Clusters in the Cubic Helimagnet $Cu_2OSeO_3$ – Supplementary Information

J. C. Loudon,[1,*] A. O. Leonov,[2,3,4,†] A. N. Bogdanov,[3,4] M. Ciomaga Hatnean,[5] and G. Balakrishnan[5]

[1]*Department of Materials Science and Metallurgy, 27 Charles Babbage Road, Cambridge, CB3 0FS, United Kingdom.*
[2]*Department of Chemistry, Faculty of Science, Hiroshima University Kagamiyama, Higashi-Hiroshima, Hiroshima 739-8526, Japan.*
[3]*Chiral Research Center, Hiroshima University, Higashi-Hiroshima, 739-8526, Japan.*
[4]*IFW Dresden, Postfach 270016, D-01171 Dresden, Germany.*
[5]*Department of Physics, University of Warwick, Coventry CV4 7AL, United Kingdom.*

(Dated: February 7, 2018)

## I. THE STRUCTURE OF SKYRMIONS WITHIN THE CONE PHASE

Here we describe in detail the structure of skyrmions embedded in the cone phase. We first describe the structure obtained by minimizing the energy functional and then compare it with a possible structure that intuition might suggest.

### A. Skyrmion Structure Obtained by Minimization of the Energy Functional

Fig. S1 shows the results of numerically minimizing of the energy functional (Eqn. (1) in main paper)

$$w = A(\mathbf{grad}\,\mathbf{M})^2 + K(\mathbf{M}\cdot\mathbf{n})^2 - \mu_0\mathbf{M}\cdot\mathbf{H} + w_D, \quad (1)$$

subject to the boundary conditions (Eqn. (2) in main paper)

$$\theta_\infty = \theta_c = \arccos\left(H/H_C\right), \, \psi_\infty = \psi_c = 2\pi z/L_D, \quad (2)$$

The asymmetry of skyrmions within the conical phase is clear in both the in-plane and $z$ components of the magnetization. Fig. S1(a) shows the magnetization in a plane normal to the direction of the applied field $z$ and (c) is a vertical linescan through the center of (a). It can be seen that these skyrmions consist of a nearly axisymmetric core surrounded by a crescent-shaped transitional region. The points $C$ and $D$ have the same $m_z$ component as the conical phase and serve to mark the limits of the axisymmetric region. The structure shown in (a) rotates on moving along $z$ from one plane to the next and $A$, the point at which $m_z = -1$ circumscribes a circle about the central axis, $B$ which has a very similar magnetization. Fig. S1(b) shows a cross-sectional view in $xz$ with the position of $A$ marked by the dash-dot line.

### B. An Intuitive Model for Skyrmions Embedded in the Cone Phase

Here we present an intuitive method to construct a skyrmion compatible with the cone phase and compare it with the result obtained by energy minimization described in the previous section. The skyrmion is constructed by starting with a conventional axisymmetric skyrmion embedded in the saturated phase shown in Fig. S2(a) and breaking it up into planes normal to the applied magnetic field. (To make the procedure more instructive, the skyrmion is a Néel type.) Then all the magnetic moments in each plane are tilted by the canting angle appropriate for the cone phase resulting in Fig. S2(b). Thus the moments far from the center lie parallel to those in the cone phase and the moment in the center is antiparallel.

Vertical linescans through the skyrmion centers are shown in Fig. S2(c) for comparison. The point $E$ in the center of the axisymmetric skyrmion becomes point $K$ with a value of $m_z$ antiparallel to the surrounding state. The magnetization has the same polar angle as the surrounding conical phase but with the opposite in-plane orientation at point $H$ and the points $G$ and $F$ are the centers of the crescent and the core, respectively.

This structure shares the main features of the skyrmion found by energy minimization shown in Fig. S1(a), notably an axisymmetric core surrounded by a crescent-shaped transitional region. The vertical line profiles through the center of the skyrmion shown in Figs. S1 (c) and S2 (c) also show similar features. This construction could be used as an initial configuration for numerical simulations.

## II. EXPERIMENTAL METHODS

$Cu_2OSeO_3$ single crystal samples of size 3 mm were grown by the vapor transport technique described in ref. 1. These showed clear facets and the sample was thinned for electron microscopy by mechanically polishing on a (110) face until it was 20 $\mu$m thick. It was then further thinned by argon ion beam irradiation using a Gatan Precision Ion Polishing System (PIPS) initially operated at 4 kV with the ion guns set at 7° to the sample plane. Once the sample thickness approached the wavelength of light, rainbow colors could be observed using an optical microscope and, at this point, the voltage was reduced to 2 kV and the gun angle to 5° and thinning

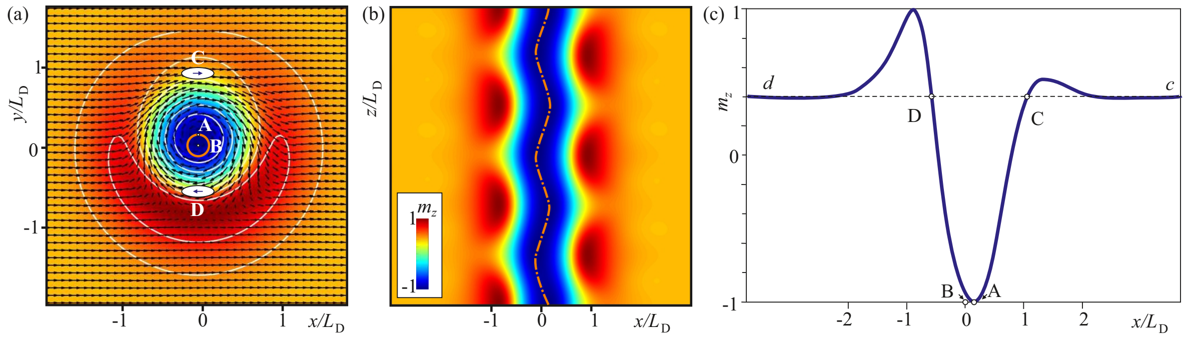


FIG. S1. (color online) The magnetic structure of a skyrmion embedded in the cone phase obtained by minimizing the energy functional (Eqn. 1). The applied magnetic field, $\mathbf{h} = 0.4$, is directed along the $z$ axis. (a) and (b): Color plots of $m_z$ in the $xy$ and $xz$ planes, respectively. The color bar in (b) applies to both panels. The in-plane components of the magnetization in (a) are shown by black arrows. (c) The $m_z$ component of the magnetization obtained from a vertical linescan through the center of (a).

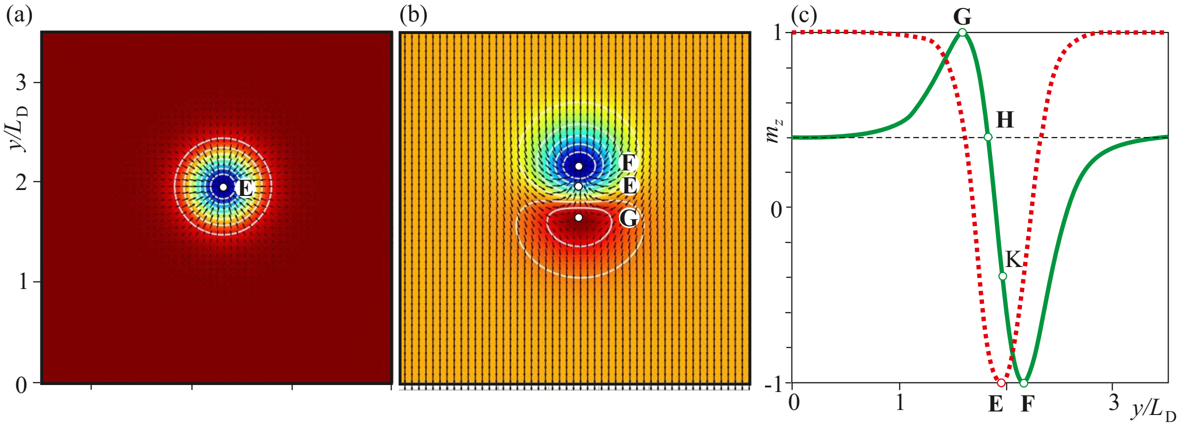


FIG. S2. (color online) Construction of a model solution for non-axisymmetric skyrmions. As an initial configuration we use a solution for axisymmetric skyrmions (a) with the surrounding field-polarized state for $\mathbf{h} = 1.1$. With the help of a rotation matrix we rotate each spin in this configuration and obtain a model solution (b). (c) The $m_z$ component of the magnetization obtained from a vertical linescan through the skyrmion center in an axisymmetric skyrmion (a) (red dotted line) and a model solution for non-axisymmetric skyrmion (b) (green solid line). We also mark different points that could be named as centers of the resulting non-axisymmetric skyrmion (see text for details).

continued until a hole of size 15 $\mu$m appeared.

Transmission electron micrographs were taken from an area of sample approximately 70 nm thick surrounding this hole with an FEI Tecnai F20 transmission electron microscope (TEM) equipped with a field-emission gun using an acceleration voltage of 200 kV. In normal operation, the objective lens of the microscope applies a 2 T field to the specimen which would force it into the saturated state. Images were instead acquired in low-magnification mode in which the image is formed using the diffraction lens and the objective lens was weakly excited to apply a small magnetic field normal to the plane of the specimen.

The sample was cooled using a Gatan liquid-helium cooled IKHCHDT3010-special tilt-rotate holder which has a base temperature of 10 K. The images were energy-filtered so that only electrons which had lost between 0 and 10 eV on passing through the specimen contributed to the image and recorded on a video-rate CCD camera at 25 frames per second. An aperture was used to ensure that only the 000-beam and the low-angle scattering from the skyrmions contributed to the image.

The defocus and magnification were calibrated by acquiring images with the same lens settings from Agar Scientific's "S106" calibration specimen which consists of lines spaced by 463 nm ruled on an amorphous film. The defocus was found by taking digital Fourier transforms of these images and measuring the radii of the dark rings that result from the contrast transfer function using the method described in ref. 2.

Magnetic phenomena can be visualized using electron microscopy as the Lorentz force from the magnetic flux in the specimen deflects the electron beam as it passes through and the magnetic structure can be seen in out-of-focus images on a scale of nanometers. Magnetic helices appear as black and white stripes and skyrmions appear

as black or white dots. Neither the cone or saturated phases produce any contrast in a defoused image.

## III. VIDEOS OF SKYRMION CLUSTERS

Video 1 corresponds to Fig. 2 of the main paper and shows two skyrmion clusters in the cone phase of $Cu_2OSeO_3$ at 11 K in an applied field of 116 mT. As with all the videos, the spacing between the skyrmions is 60 nm and the video is shown in real time. All the videos were taken under very similar conditions from different regions of the sample.

Video 2 shows two more skyrmion clusters recorded at 12 K and 116 mT.

Video 3 corresponds to Fig. 3 of the main paper and shows a skyrmion cluster joining the skyrmion lattice at 12 K and 116 mT.

Video 4 shows another skyrmion cluster joining the skyrmion lattice in a different region of the sample to video 3 under the same conditions.

---

* j.c.loudon@gmail.com
† leonov@hiroshima-u.ac.jp

[1] S. Seki, X. Z. Yu, S. Ishiwata, and Y. Tokura, "Observation of skyrmions in a multiferroic material," Science **336**, 198 (2012).
[2] D. B. Williams and C. B. Carter, *Transmission Electron Microscopy* (Springer, New York, 1996) Chap. 28.
